# Supplementary material for: What Changed and What Could Have Changed? State-Change Counterfactuals for Procedure-Aware Video Representation Learning
Source: arXiv:2503.21055 source file (2025-08-12)
Supplement: Supplementary file 2 [file qualitative_results.tex]

% \subsection{Full Results of Action Phase Classification \& Retrieval}
% \label{subsec:full}
% Tables \ref{table:ae2_cls} and \ref{table:ae2_retrieval} show classification and retrieval results on the Align-Ego-Exo~\cite{xue2023learning} dataset for each activity.

% \subsection{Qualitative Results}
% \label{sub}
% \begin{figure*}[t!]
% \centering
%         % \rule{0.8\textwidth}{5cm}
%         \includegraphics[width=17cm]{Figure/q1.pdf}
%         % \rule{0.8\textwidth}{5cm}
%         % \vspace{-1mm}
%         \caption{
%                  Qualitative results of Error Detection on EgoPER. GT denotes ground truth. \textcolor{OliveGreen}{Green}/\textcolor{red}{Red} segmentation and text denote the normal and error labels, respectively. The presented erroneous procedure \emph{``Make tea''} consists of [\emph{``\textcolor{red}{Not checking water temperature in the kettle},''} \emph{``\textcolor{OliveGreen}{{Hold the kettle,}}'' \emph{\textcolor{red}{``Pour water immediately,''} }\emph{\textcolor{red}{``Stir with the knife'',}} ....}].
%                  } 
        
%         \label{fig:qualitative}
%         \vspace{4mm}
% \end{figure*}


% \begin{figure*}[t!]
% \centering
%         % \rule{0.8\textwidth}{5cm}
%         \includegraphics[width=17cm]{Figure/q2.pdf}
%         % \rule{0.8\textwidth}{5cm}
%         % \vspace{-1mm}
%         \caption{
%                 Qualitative results of Temporal Action Segmentation on EgoPER. The example presents the procedure \emph{``Make Pinwheel''}. Distinct colored segments are different action step classes.
%                  } 
        
%         \label{fig:qualitative_2}
%         \vspace{3mm}
% \end{figure*}

% Figure~\ref{fig:qualitative} presents qualitative results on error detection in EgoPER, showing that our learned representations identify erroneous activities with greater fidelity. PVRL and HierVL produce several false positives, leading to over-segmentation, whereas our method better aligns with the ground-truth segments in both temporal location and count. 
% % 
% Figure~\ref{fig:qualitative_2} shows qualitative results on Temporal Action Segmentation, where PVRL and HierVL misclassify large temporal segments (dark and light orange, respectively). In contrast, our model more accurately distinguishes and classifies actions, reflecting an improved understanding of procedural activities and aligning with our quantitative results.
