# Supplementary material for: What Changed and What Could Have Changed? State-Change Counterfactuals for Procedure-Aware Video Representation Learning
Source: arXiv:2503.21055 source file (2025-08-12)
Supplement: Supplementary file 3 [file text_generation.tex]

% \clearpage
% \setcounter{page}{1}
% \maketitlesupplementary

\section{Text Generation}
\label{sec:rationale}

\hank{generation details}

\hank{generation examples}
